# Supplementary material for: NeurOCS: Neural NOCS Supervision for Monocular 3D Object Localization
Source: arXiv:2305.17763 source file (2023-05-28)
Supplement: Supplementary file 1 [file additionaldetails.tex]

\section{Supportive Explanations}

\noindent \textbf{NeRF grid configurations.} \label{sec:nerf_details}
Our NeRF representation rests on latent feature grids that can be efficiently decoded into color and density with a small MLP.
We use the implementation from \cite{tiny_cuda_nn} for latent grids that correspond to the space of a unit cubic. 
%We use a base width of 2 with 5 multi-scales and increase the width 2 times at each scale. This results in a maximum of grid resolution of $32 \!\times\! 32 \!\times\! 32$ at finest scale. 
In particular, we adopt the multi-resolution representation consisting of five latent grids, each with size $(2{\times}2{\times}2)$, $(4{\times}4{\times}4)$, $(8{\times}8{\times}8)$, $(16{\times}16{\times}16)$, and $(32{\times}32{\times}32)$. Each vertex on the grid stores a 4-dimensional learnable feature vector.
%Grid at each scale stores a 4-vector feature, 
Given a sampled point inside the 3D object box, we use its size-normalized NOCS to query each latent grid by trilinear interpolation, resulting in a total of $5{\times}4{=}20$ dimensional feature vector after concatenation. The feature vector is passed to an MLP containing three 64-channel hidden layers with ReLU activation, yielding color and density. We illustrate this procedure in \cref{fig:supp_gridnerf}, with two resolution scales for clarity of visualization. For each batch iteration during training, we randomly sample 768 rays per object to enforce rendering losses.

\begin{figure}[!t]
    \centering
    \includegraphics[width=1.0\linewidth, trim = 0mm 38mm 60mm 0mm, clip]{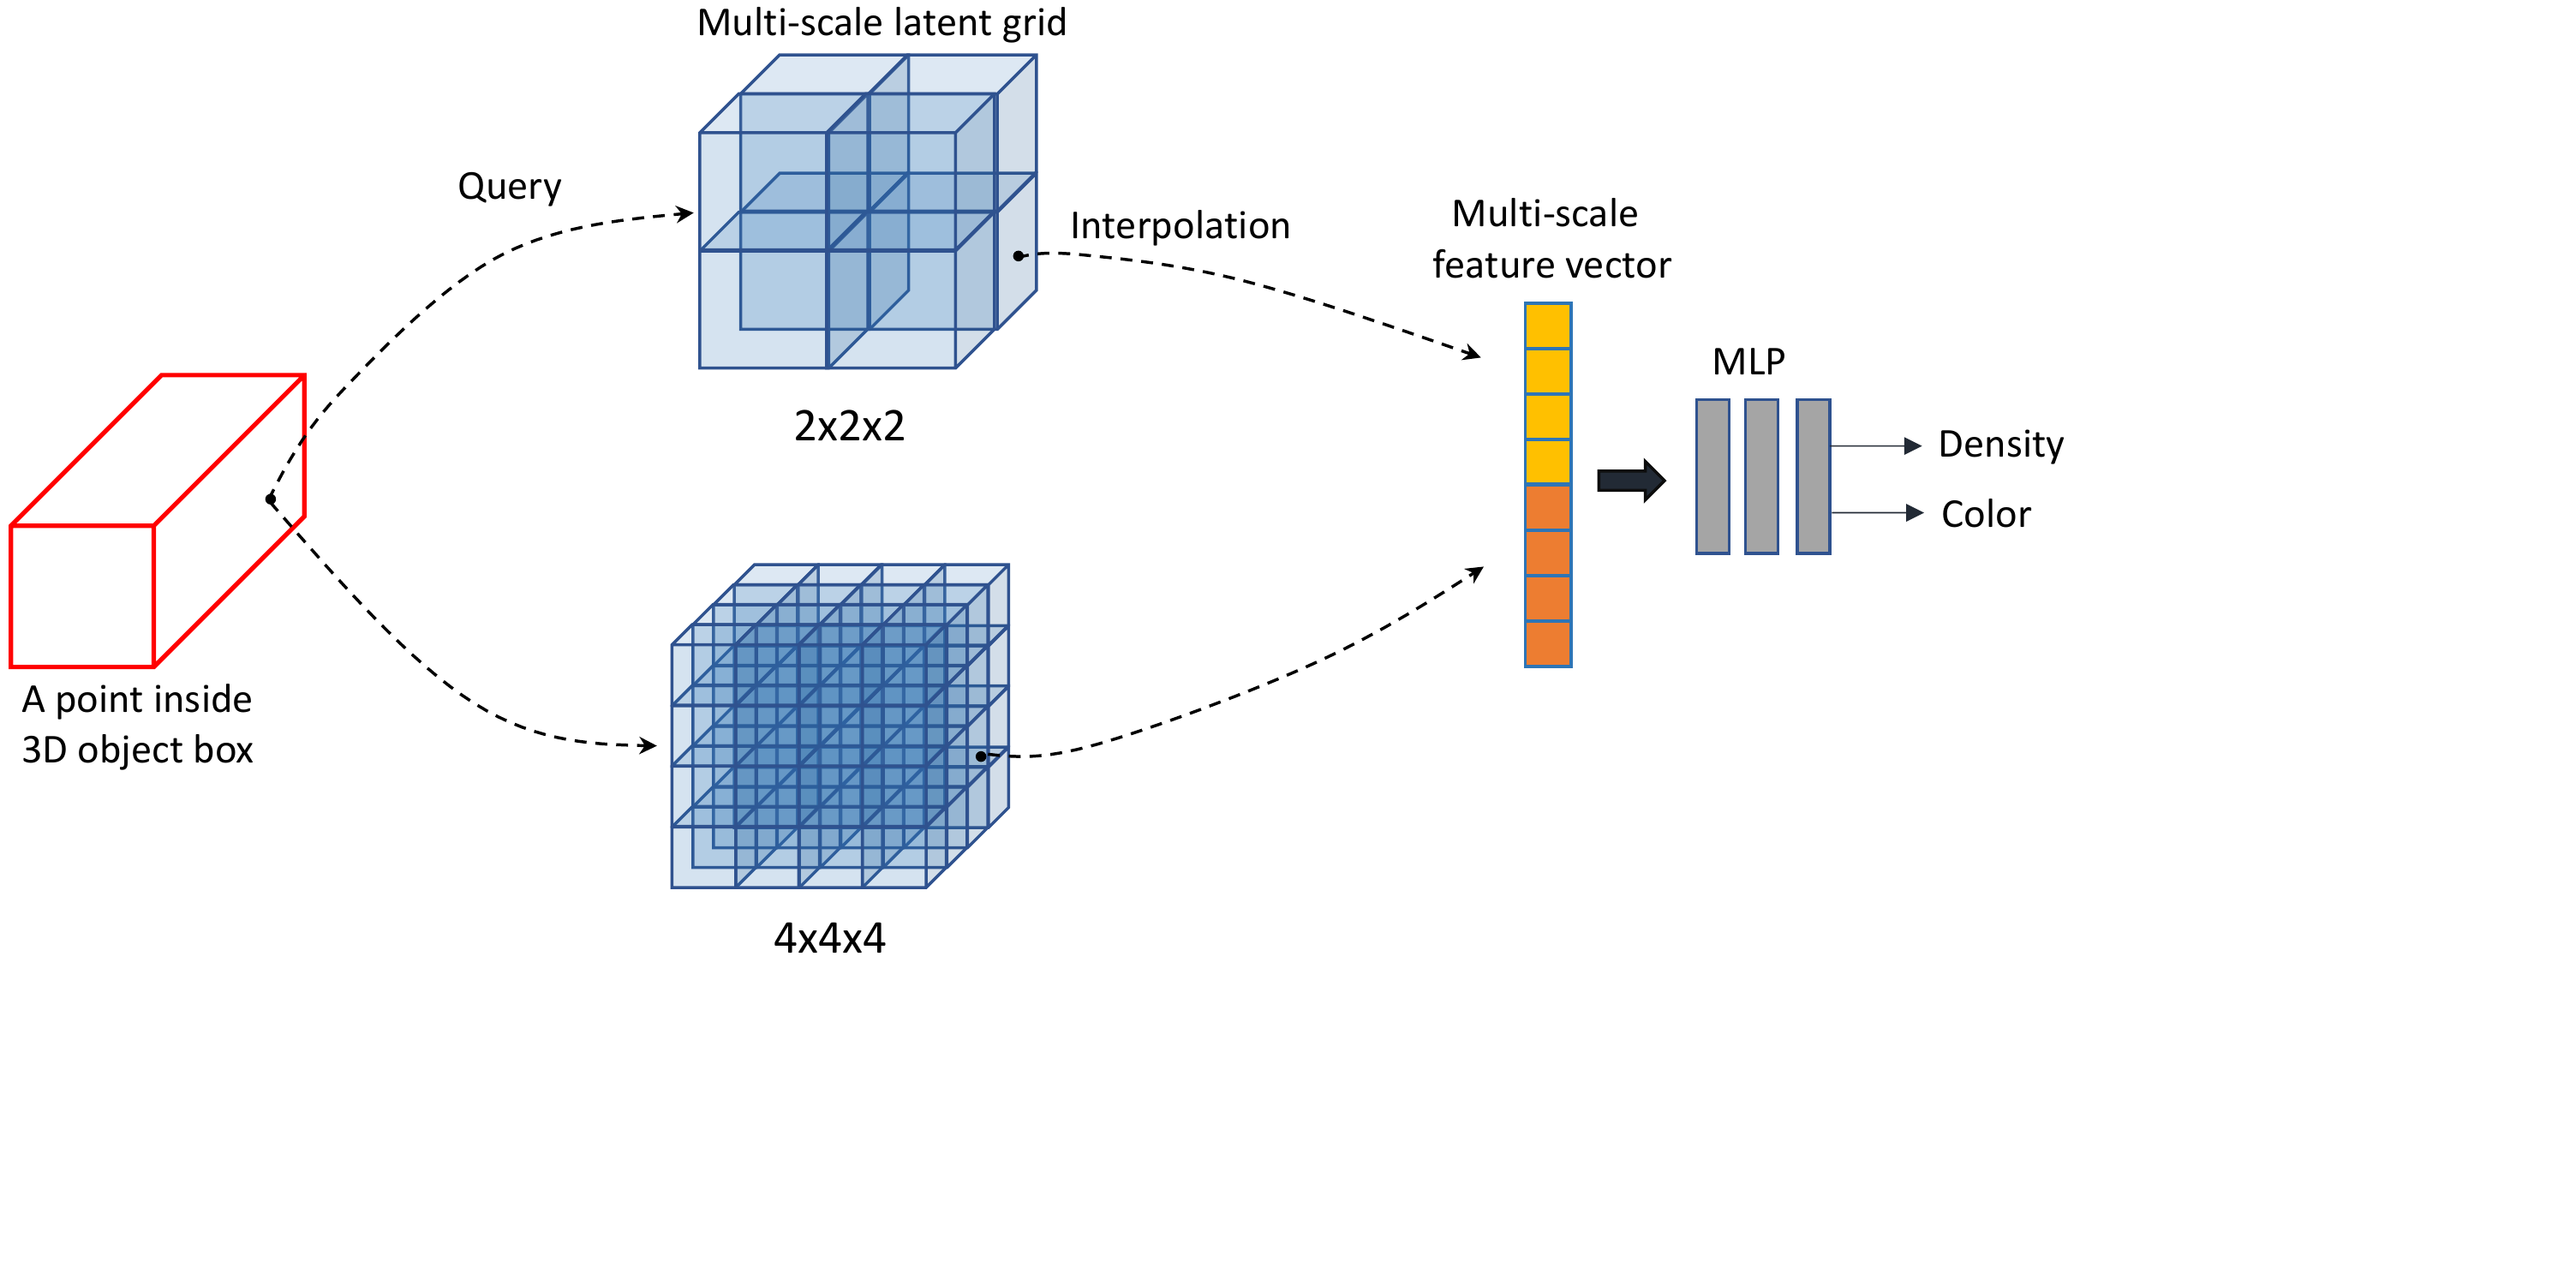}
    \caption{\textbf{Illustration of our grid NeRF} that decodes color and density from a feature vector queried from latent grids. We use latent grids with five scales but only two are visualized for clarity.  }
    \label{fig:supp_gridnerf}
\end{figure}

\begin{figure}[!t]
    \centering
    \includegraphics[width=1.0\linewidth, trim = 0mm 0mm 10mm 0mm, clip]{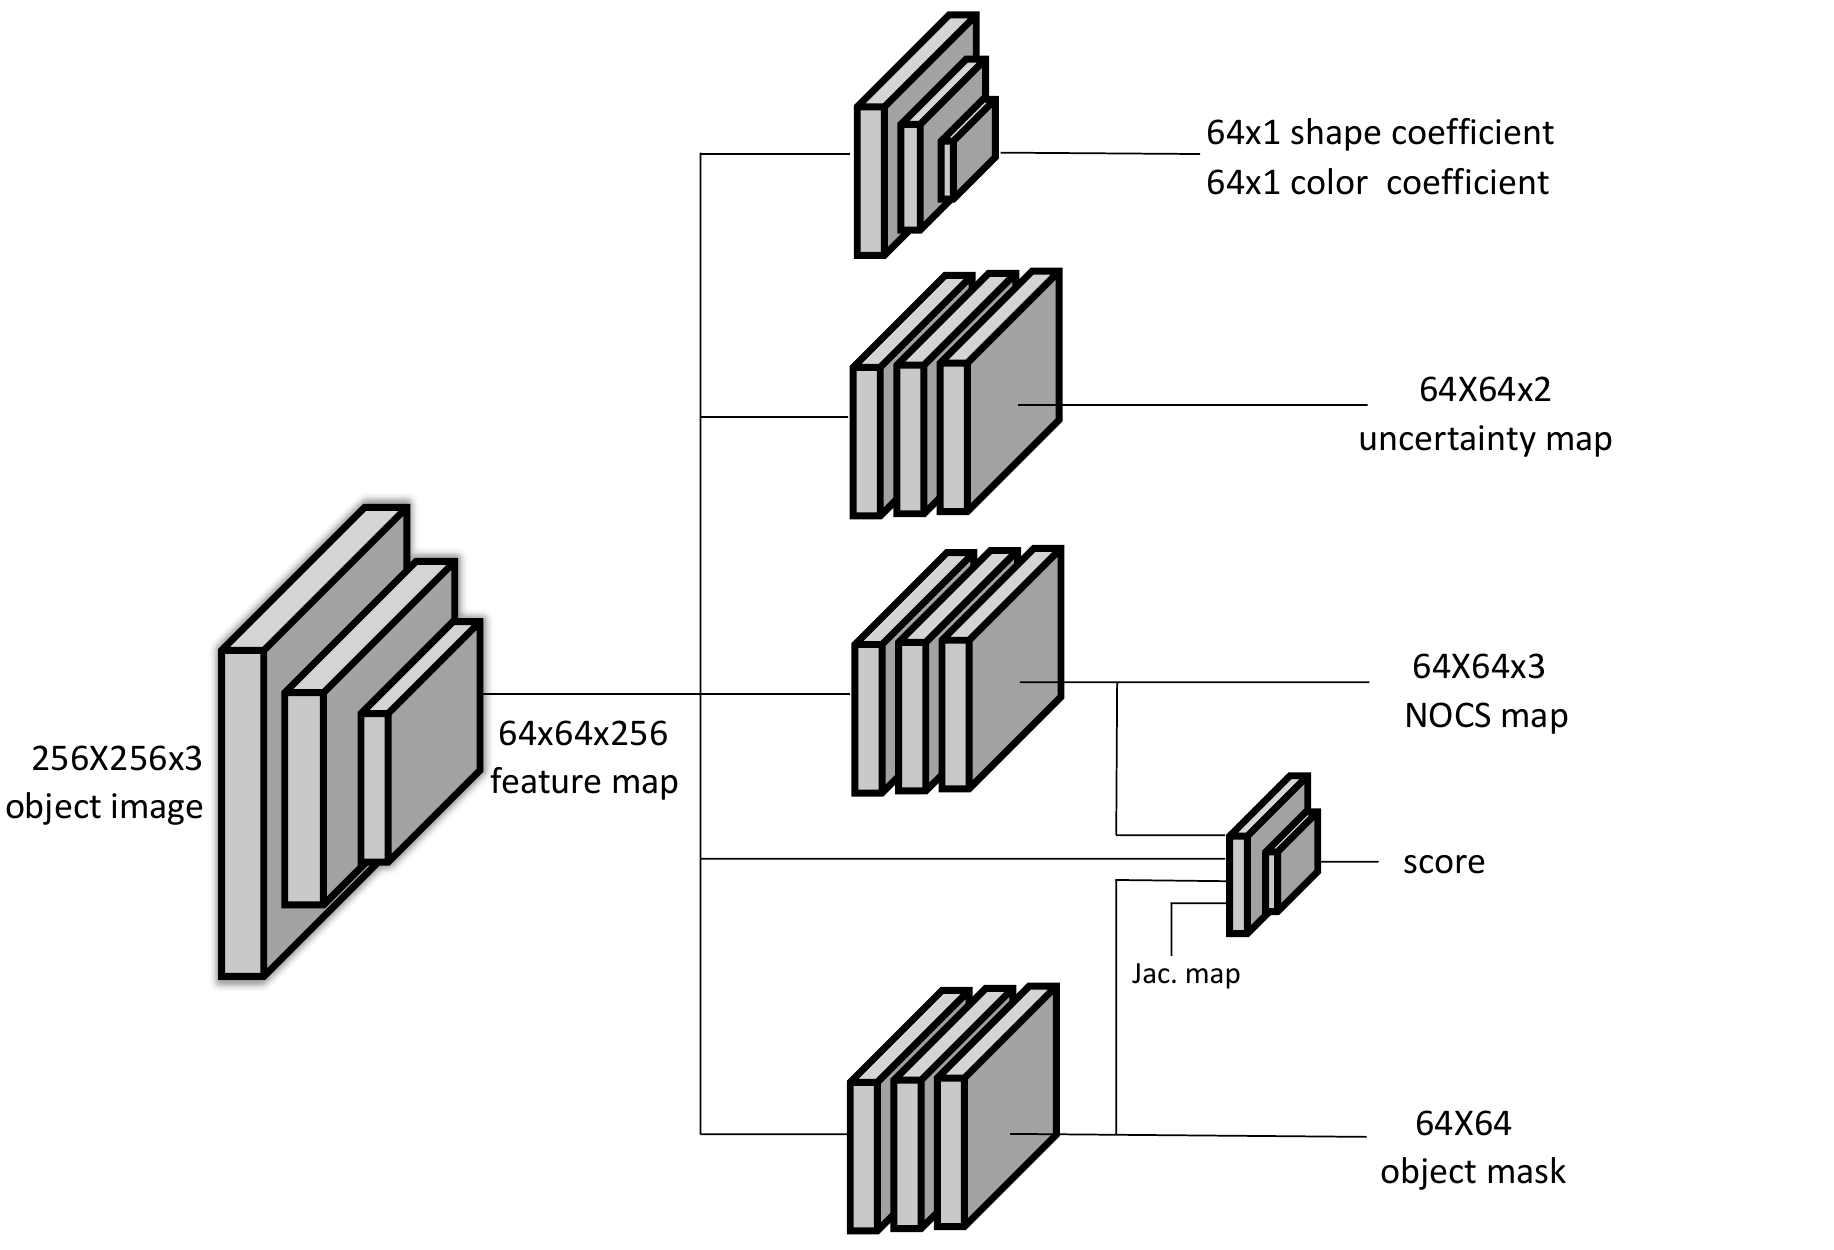}
    \caption{\textbf{Structure of our image-conditioned network} consisting of a backbone feature extraction network and a number of regression heads for different predictions.  
    }
    \label{fig:supp_network}
\end{figure}

\vspace{0.1cm}
\noindent \textbf{Base 3D detector.} It is worth stressing that the training of NeurOCS is agnostic to the base 3D detector -- NeurOCS takes ground truth 2D boxes as input in training, and during inference it is combined with a base 3D detector of choice, taking its 2D boxes as input. Also note the object size prediction is not needed during training. This makes  NeurOCS a standalone NOCS-based framework that can be flexibly combined with different base 3D detectors. In addition to DID-M3D, we show in next section that it also works well with another state-of-the-art 3D detector DEVIANT~\cite{kumar2022deviant}. As future work, we envision that NeurOCS has potential to improve Lidar-based 3D detection as well.

\vspace{0.1cm}
\noindent \textbf{Network architecture.} We illustrate our network pathways in \cref{fig:supp_network}. 
%We use ResNet50 pretrained on ImageNet as backbone. 
We crop objects using 2D boxes and resize to $256\!\times\!256$ as input to our backbone network, a ResNet50 pretrained on ImageNet. We extract its  $8{\times}8$ feature map at the fourth layer, upsample to $64{\times}64$ by bilinear interpolation, and then pass to a few regression heads. We apply three separate heads to predict the NOCS map, the uncertainty map (detailed later), and the foreground object mask, each using three $1{\times}1$ convolutional layers with BachNorm and ReLu activation.
The shape and color coefficients are predicted by a 3-layer MLP with the average-pooled feature map as input. The score prediction head uses two $1\!\times\!1$ convolutional layers followed by average-pooling and a linear layer to regress a confidence score. It takes as input the object feature map, the predicted NOCS map, the predicted foregound object mask, and the Jacobian map.

\begin{figure}[!t]
    \centering
    \includegraphics[width=1.0\linewidth, trim = 0mm 80mm 0mm 0mm, clip]{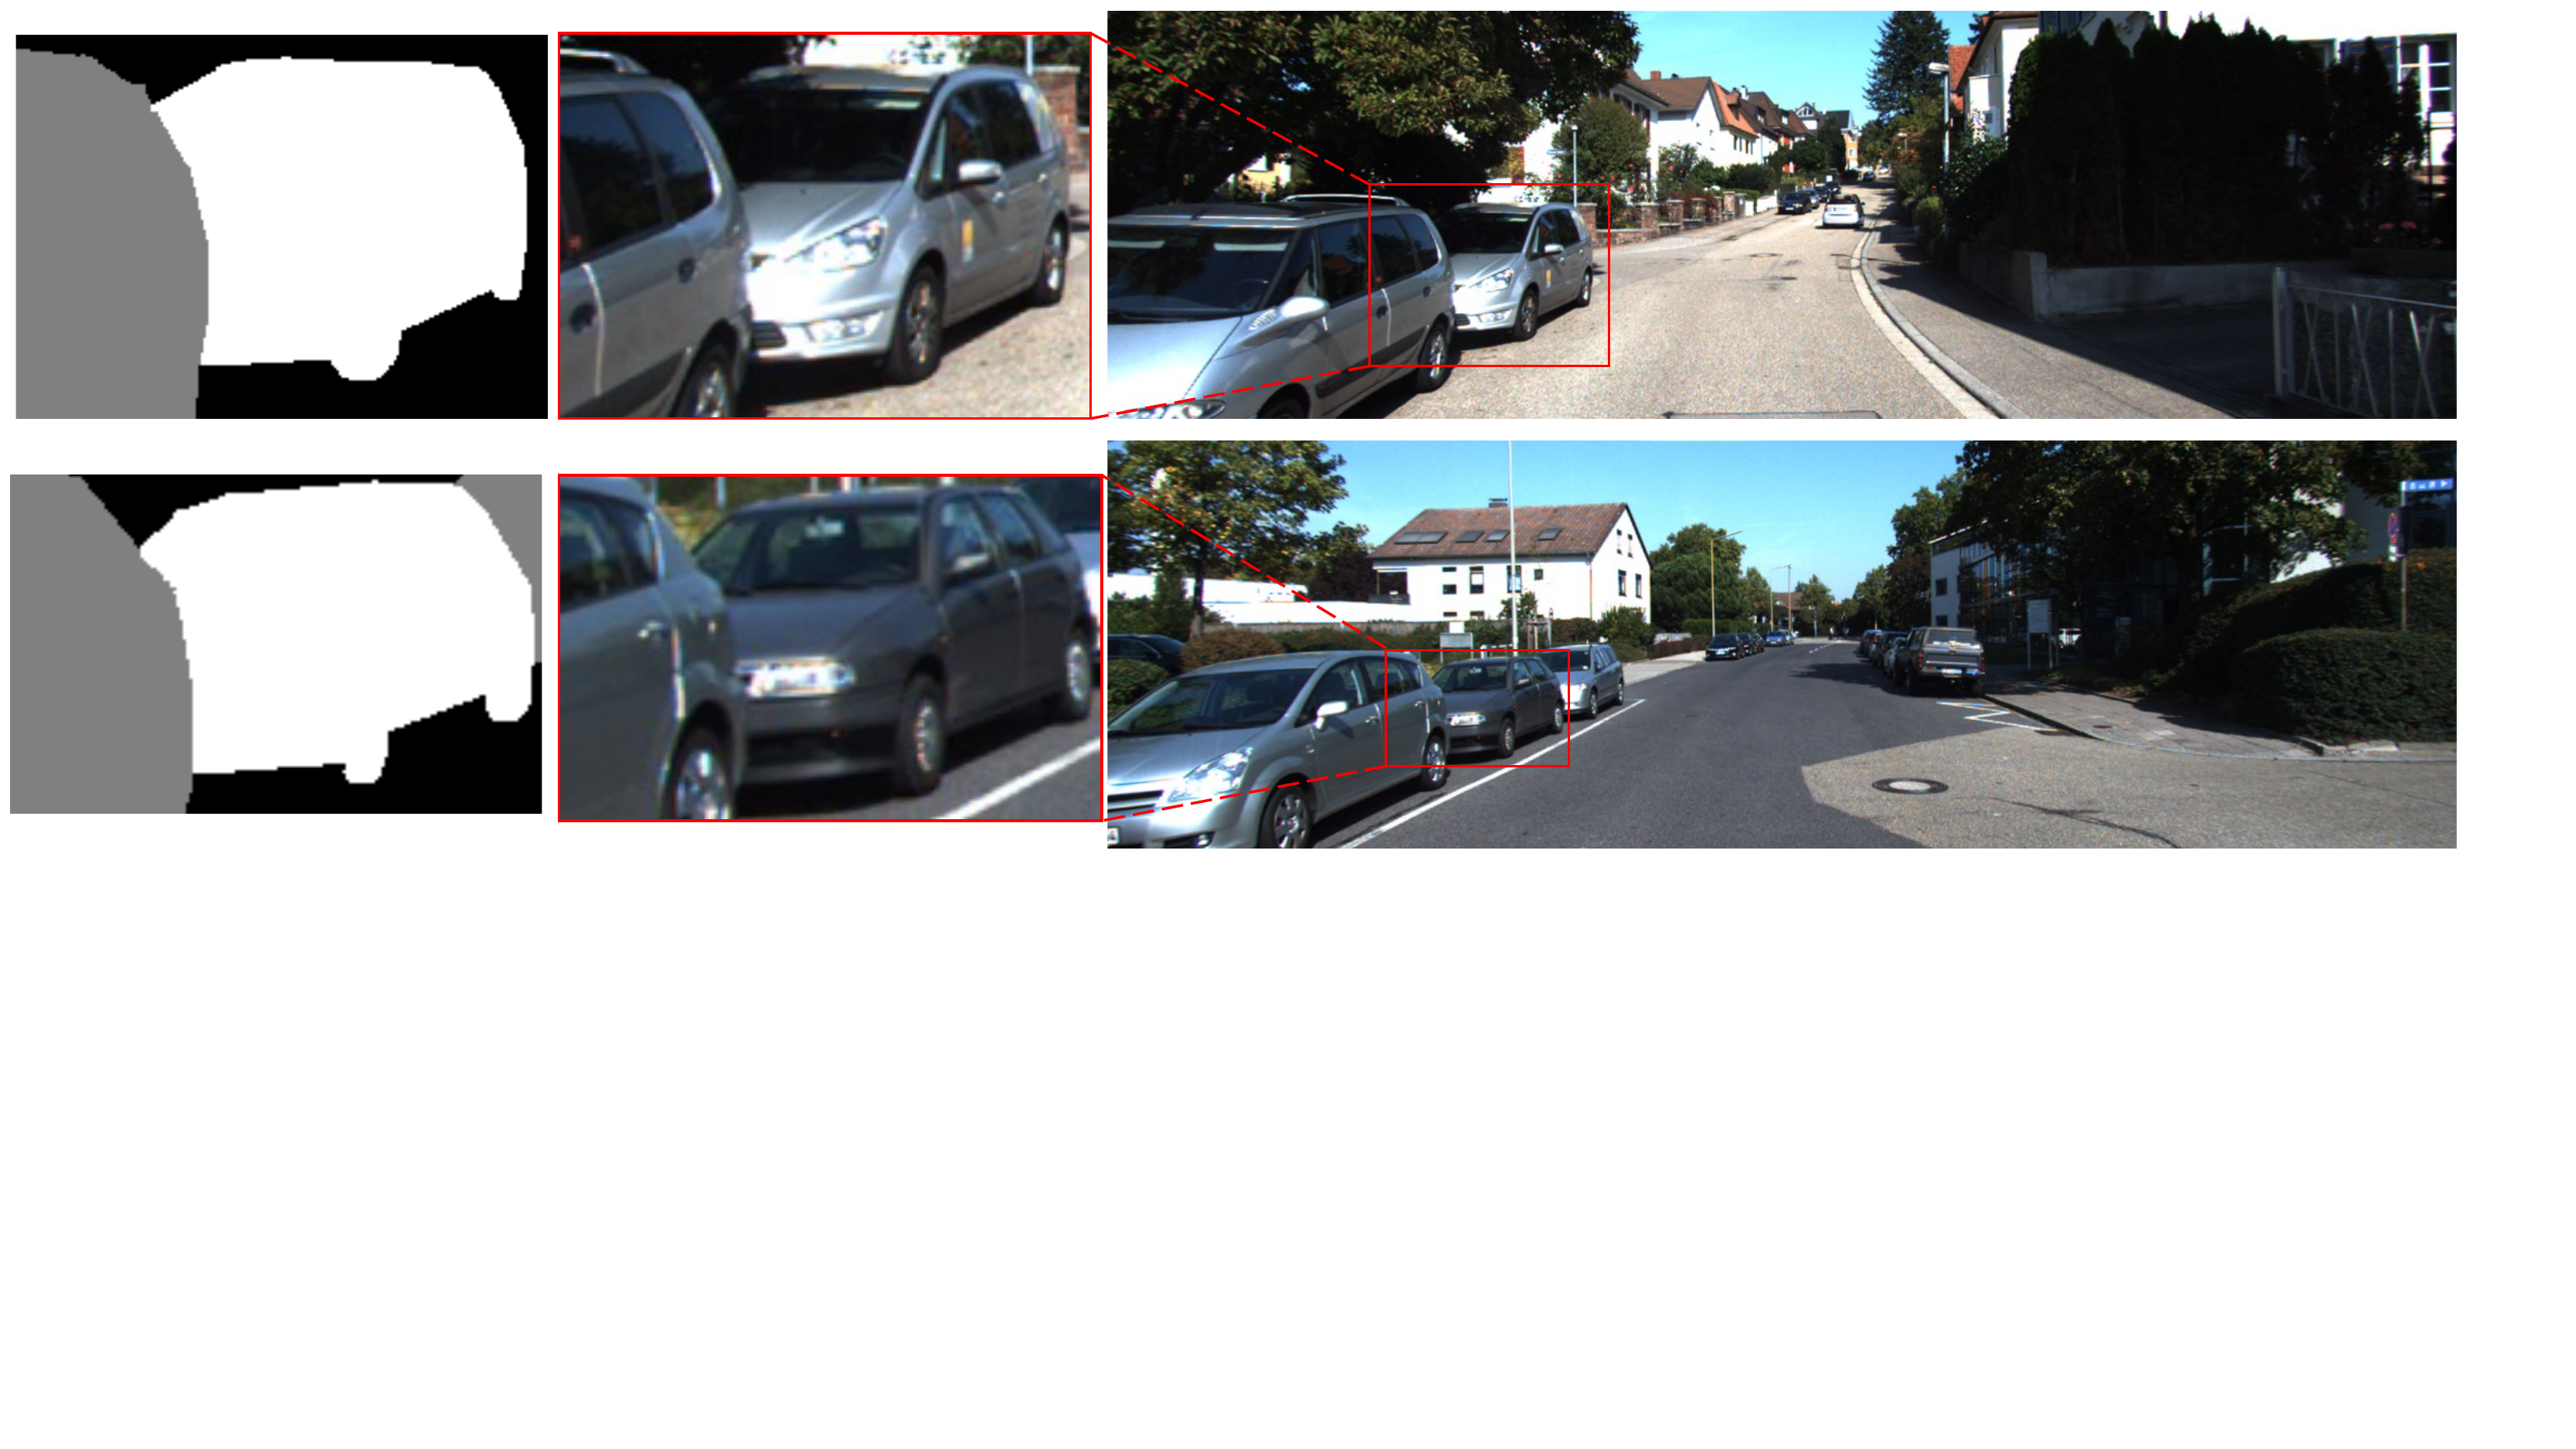}
    \caption{\textbf{Illustration of our ground-truth object mask.} The white, black, and gray pixels indicate foreground, background, and unknown regions, respectively.}
    \label{fig:supp_objectmask}
\end{figure}

\vspace{0.1cm}
\noindent \textbf{Foreground object masks.} We demonstrate our ground-truth object mask with two example objects in \cref{fig:supp_objectmask}. The foreground and background regions provide shape constraints in our occupancy loss akin to the machinery of shape-from-silhouette. Pixels on other object instances are ignored as they are likely occluding objects that obscure the shape boundary.

\begin{table}
    \centering
    
    \resizebox{0.9\columnwidth}{!}{%
        \begin{tabular}{c|c|c|c|c|c}
\hline
Module & Loss Name & Type & Weight & Region & Note \\ \hline
\multirow{6}{*}{NeRF} & Occupancy Loss & L2 & 1 & FG + BG &  \\
 & RGB Loss & L2 & 3 & FG &  \\
 & KL Divergence & KL & 1 & - &  \\
 & Lidar Loss & L2 & 0.5 & FG \& Valid & Optional \\
 & LiComp Loss & L2 & 0.2 & FG \& Valid & Optional \\
 & Dense Prior & L1 & 0.002 & 3D Grid & Conditional \\ \hline
\multirow{3}{*}{Image} & FG Loss & L2 & 1 & All &  \\
 & IoU Score Loss & L2 & 1 & - &  \\
 & Reproj. Loss & L2 & 2 & FG &  \\ \hline
Both & NOCS Consistency & L2 & 1 & FG \& Occ &  \\ \hline

\multicolumn{6}{r}{\small {FG = Foreground, \; BG = Backgroud}}

\end{tabular}
    }
    \caption{\textbf{A summary of our losses}, including NeRF losses and image-conditioned regression losses. See text for details.  }
    \label{table:losses}
\end{table}

\vspace{0.1cm}
\noindent \textbf{Shape Regularization}. We demonstrate the impact of the KL divergence loss in \cref{fig:visual_hull_ambiguity}(a), illustrate the visual hull ambiguity and that the dense prior improves the shape \cref{fig:visual_hull_ambiguity}(b).

\vspace{0.1cm}
\noindent \textbf{Loss.} We jointly train the image-conditioned regression network and the NeRF by combining all their losses. In \cref{table:losses}, we detail the training losses composition, including their weight, application scope and  condition. 
%The occupancy, FG, RGB and reprojection losses are normalized to $[0,1]$ (w/o square). 
%The NOCS consistency, Lidar, LiComp losses computes the difference between NOCS, hence range in $[0,2]$ (w/o square). 
The occupancy loss is applied on foreground and background, while skipping unknown regions. The RGB loss is only applied to the foreground region. If a point from Lidar or its completion resides inside the object 3D box and projects to the foreground region, it induces a valid NOCS point for supervision. The dense prior loss is applied to randomly sampled points inside the 3D latent grid; and it is  only applied in absence of Lidar/LiComp losses, hence marked as conditional. 
The NOCS consistency loss is applied to foreground regions and weighted by a detached occupancy map rendered from NeRF. 
We also add an unsupervised reprojection loss~\cite{chen2021monorun}, and similarly to~\cite{chen2021monorun} we learn a per-pixel aletoric uncertainty map $(\sigma_x,\sigma_y)$ for the NOCS projection on image in both horizontal and vertical diction, by optimizing $\frac{|\Delta p_x|^2}{\sigma_x^2}+\log\sigma_x^2$, where $|\Delta p_x|^2$ indicates the reprojection error in $x$ direction; same applies to $\sigma_y$. The confidence $(\frac{1}{\sigma_x},\frac{1}{\sigma_y})$ is multiplied with the foreground probability to weigh each pixel in PnP optimization, which also optimizes the reprojection error loss.
The weights combining the losses are chosen empirically based on the validation set, and we note that the performance is not sensitive to these parameters in practice.

\noindent \textbf{Data augmentation.} During the training, we apply data augmentation on the ground truth 2D boxes, including flipping and bounding box perturbation similar to~ \cite{li2019cdpn}.

\begin{figure}[t]
    \centering
    \includegraphics[width=\columnwidth]{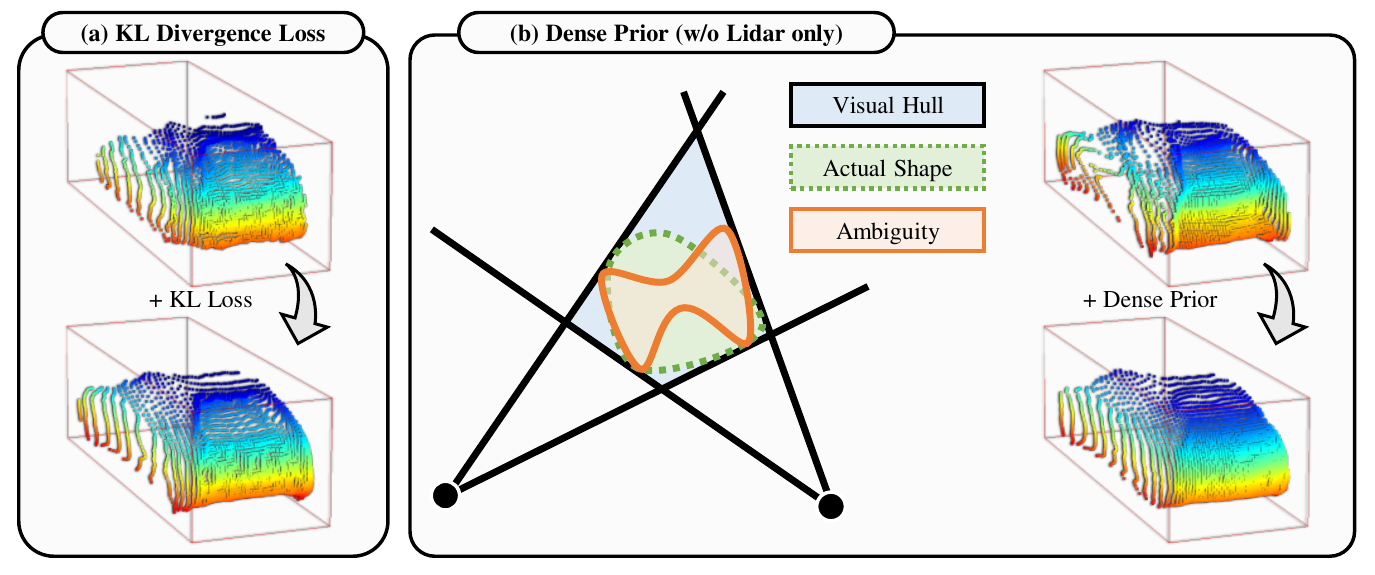}
    \caption{\textbf{Shape Regularizations.} (a) An actual example showing the KL loss yields cleaner shape. (b) An illustration on the visual hull ambiguity and the impact of the dense shape prior.
    }
    \label{fig:visual_hull_ambiguity}    
\end{figure}
