# Supplementary material for: NeurOCS: Neural NOCS Supervision for Monocular 3D Object Localization
Source: arXiv:2305.17763 source file (2023-05-28)
Supplement: Supplementary file 2 [file additionalexp.tex]

\section{Additional Experimental Results}

\subsection{Additional Results on KITTI}

\begin{table}
    \centering
    
    \resizebox{1.0\columnwidth}{!}{%
        \begin{tabular}{c|c|lll|lll}
\multirow{2}{*}{Method} & \multirow{2}{*}{Venue} & \multicolumn{3}{c|}{3D $AP_{40} $ - Val} & \multicolumn{3}{c}{BEV $AP_{40} $ - Val} \\ \cline{3-8} 
                        &                        & Easy       & Mod      &Hard      & Easy      & Mod      & Hard      \\ \hline
DEVIANT~\cite{kumar2022deviant}  & ECCV22 &  25.09 & 16.99 & 15.30 & 33.69 & 23.10 & 20.67           \\\hline
%NeurOCS-M   & - & 22.71 & 15.78 & 14.01 & 29.32 & 21.40 &  18.79 \\
%NeurOCS-MLC  & - & 21.98& 15.73 & 13.79 & 29.33 & 21.22 & 18.64 %\\\hline    
NeurOCS-M + \cite{kumar2022deviant}  & CVPR23 & 27.70 & 18.92 & 16.28 & 35.31 & 25.11 & 21.87 \\        
NeurOCS-MLC + \cite{kumar2022deviant}  & CVPR23 & 27.83 & 18.92 & 16.20 & 35.14 & 24.77 & 21.43 \\        
\end{tabular}

    }
    \caption{Evaluation with DEVIANT~\cite{kumar2022deviant} as our base 3D detector.}
    \label{table:comparewith_deviant}
\end{table}

\begin{table}
    \centering
    
    \resizebox{1.0\columnwidth}{!}{%
        \begin{tabular}{l|c|lll|lll}
\multirow{2}{*}{Method} & \multirow{2}{*}{Venue} & \multicolumn{3}{c|}{3D $AP_{40} $ - Test} & \multicolumn{3}{c}{BEV $AP_{40} $ - Test} \\ \cline{3-8} 
                        &                        & Easy       & Mod      & Hard      & Easy      & Mod      & Hard      \\ \hline
                      LPCG~\cite{peng2022lidar}  & ECCV22 & 25.56 & 17.80 & 15.38 & 35.96 & 24.81 & 21.86  \\
                      CMKD~\cite{hong2022cross} & ECCV22 & 28.55 & 18.69 & 16.77 & 38.98 & 25.82 & 22.80 \\
                      NeurOCS  & CVPR23 &  29.89 & 18.94 & 15.90 & 37.27 & 24.49 & 20.89
\end{tabular}

    }
    \caption{Additional comparison with LPCG~\cite{peng2022lidar} and CMKD~\cite{hong2022cross} on KITTI test set. }
    \label{table:comparewith_cmkd}
\end{table}

\noindent \textbf{Base 3D detector.} We demonstrated good performance with DID-M3D~\cite{peng2022did} as our base 3D detector in the main paper. Here, we evaluate performance by combining NeurOCS with another base 3D detector, namely DEVIANT~\cite{kumar2022deviant}. As can be seen in \cref{table:comparewith_deviant}, NeurOCS improves over DEVIANT with the scale fusion, whether the shape is trained with mask only or with additional Lidar supervision. This further consolidates the value of NeurOCS as a standalone shape-based 3D localization framework. 

\if false
\begin{figure}
    \centering
    \includegraphics[width=\columnwidth]{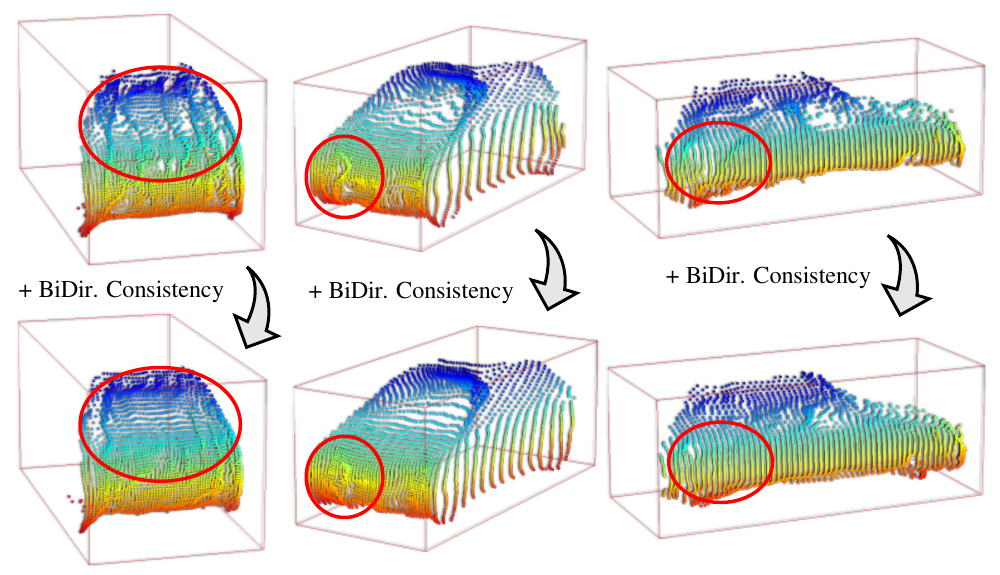}
    \caption{Three object instances demonstrating that the bi-directional NOCS consistency yields slightly smoother and better shapes.}
    \label{fig:bidir}
\end{figure}
\fi

\noindent \textbf{Additional comparison on KITTI benchmark.} In the main paper, we primarily compare with existing methods that rely on the original 3D box annotations from KITTI to train the 3D detector. However, it is also worth discussing recent works LPCG~\cite{peng2022lidar} and CMKD~\cite{hong2022cross} that improve performance by leveraging additional pseudo ground truth from extra large-scale unlabeled sequences with Lidar. %The pseudo ground truth is given by Lidar-based inference which further constrains the outputs from image-based networks during training.
While this line of work is orthogonal to ours, we provide performance comparison in \cref{table:comparewith_cmkd}. As shown, the accuracy from NeurOCS is superior to LPCG and comparable to CMKD.
%NeurOCS outperforms CMKD if they are trained with the original annotations, while CMKD achieves slightly better results if using the additional Lidar-based pseudo ground truth. It is important to note that our key contributions in NeurOCS are orthogonal to the advancements in the base 3D detector, \eg by leveraging unlabeled data as in CMKD, and both of them contribute to the final improvement in 3D localization, as we have shown.

\noindent \textbf{w/o NeRF results.} In the main paper, we have compared the PnP results from our NeRF-based method against directly training with raw depth supervision from Lidar and its completion w/o NeRF. Here, we report in \cref{table:withoutnerf} the full $AP_{3D}$ for the ``w/o NeRF" setting including the results after scale fusion. Note that we always include the reprojection error loss as it was shown helpful~\cite{chen2021monorun} for NOCS learning. As can be seen, the direct training yields good performance thanks to the efficacy of our framework, but lags behind the results when NeRF is applied to serve as a bridge between the raw Lidar data and the NOCS network.

\begin{table}
    \centering
    
    \resizebox{1.0\columnwidth}{!}{%
        % Please add the following required packages to your document preamble:
% \usepackage{multirow}

\begin{tabular}{l|ccc|ccc}
\hline
 \multicolumn{1}{c|}{\multirow{2}{*}{}}                               & \multicolumn{3}{c|}{PnP Only}                                       & \multicolumn{3}{c}{+ Fusion}                                       \\ 
 \multicolumn{1}{c|}{}                                                & Easy                 & Moderate             & Hard                  & Easy                 & Moderate             & Hard                 \\ \hline
 RLC & 27.55 & 18.27 & 15.75 & 30.79 & 20.78 & 17.37   \\ 
 RL &  27.50 & 18.36 & 15.77 & 30.45 & 20.71 & 17.45 \\ 
 RC &  27.08 & 18.10 & 15.28 & 30.74 & 20.67 & 17.41 \\ 
 R &   22.59 & 15.81 & 13.07 & 27.26 & 19.10 & 16.48\\
 \hline
\end{tabular}
}
    \caption{$AP_{3D}$ from directly training with raw depth supervision from Lidar and its completion w/o NeRF.}
    \label{table:withoutnerf}
\end{table}

\noindent\textbf{Network architectures.}
We study the performance with different backbone network architectures and different NeRF configurations. Our default setup uses ResNet50 and the grid NeRF with five resolution scales as described in \cref{sec:nerf_details}.
We first change ResNet50 to ResNet18 and ResNet34, only observing slightly degraded performance. This indicates NeurOCS does not heavily rely on powerful backbone, and a lighter backbone is viable in  latency-sensitive applications.
%The runtime performance trade-off is detailed in \cref{sec:supp_runtime}. 
Next, we reduce the number of NeRF scales to 4 (finest scale with $16\!\times\!16\!\times\!16$ grids) and 3 (finest scale with $8\!\times\!8\!\times\!8$ grids), where the performance %degrades slightly.
remains good. We further substitute the grid-based NeRF to a MLP-based NeRF with positional encoding same as \cite{jang2021codenerf}. In practice, we observe the MLP-based NeRF leads to nearly two times slower training process and higher memory occupancy due to its large MLP network, while the performance drops slightly.
%its performance is similar to a 3-scale grid NeRF.
\begin{table}
    \centering
    
    \resizebox{1.0\columnwidth}{!}{%
        \begin{tabular}{c|c|ccc|ccc}
\hline
\multirow{2}{*}{Module} & \multirow{2}{*}{Model} & \multicolumn{3}{c|}{PnP Only} & \multicolumn{3}{c}{+ Fusion} \\ \cline{3-8} 
 &  & Easy & Moderate & Hard & Easy & Moderate & Hard \\ \hline
 \multirow{1}{*}{Default} & ResNet50+5 Grid Scales & 27.92 & 18.49 & 15.78 & 31.24 &21.01 & 17.70 \\ \hline
 \multirow{2}{*}{Backbone} & ResNet18 & 27.04 & 18.21 & 15.39 & 30.18 & 20.80 & 17.44 \\
 & ResNet34 & 27.00 & 18.19 & 15.47 & 30.39 & 20.71 & 17.38\\ \hline
\multirow{3}{*}{NeRF} & 4 Grid Scales & 27.80 & 18.49 & 15.81 & 30.93 & 20.90 & 17.56\\
 & 3 Grid Scales & 28.02 & 18.62 & 15.89 & 31.16 & 21.02 & 17.64\\
 & CodeNeRF & 27.41 & 18.23 & 15.10 & 30.53 & 20.77 & 17.45  \\ \hline
\end{tabular}
    }
    \caption{Evaluation with $AP_{3D}$ on different backbone network architectures and NeRF configurations.}
    \label{table:supp_ablation_network_arch}
\end{table}

\noindent \textbf{Scale fusion.} In the main paper, our scale fusion is described as an averaging between scales in PnP and network-predicted object depth. In fact, we have studied the generic linear combination of the two, \ie,
%We generalize the scale fusion used in main paper by adding a linear fusion weight $w$ as
\begin{equation}
\begin{gathered}
    \mathbf{s}' =  \frac{w \cdot d_{pred}+ (1-w)\cdot[\mathbf{t}]_z}{2\cdot[\mathbf{t}]_z}\,\mathbf{s}. 
    \\
    \mathbf{t}' = \frac{w \cdot d_{pred}+ (1-w)\cdot[\mathbf{t}]_z}{2\cdot[\mathbf{t}]_z}\,\mathbf{t}.
\end{gathered}
\end{equation}
%where larger $w$ indicates the scale is relying more from direct depth estimation $d_{pred}$, while lower $w$ relying more on the PnP depth $[\mathbf{t}]_z$ estimated from the object size prediction $\mathbf{s}$.
where $w$ is a balancing weight.
%The main paper defaults $w$ to 0.5. 
We study different weight values in \cref{fig:fusew}, and empirically found 0.5 (\ie averaging) gives the overall best result, which indicates similar reliability for direct depth prediction and object size prediction that gives the metric scale in PnP solutions. We have also attempted to learn the fusion using networks akin to \cite{li2022diversity}, but found this scheme to be superior in practice.
%In Fig.\ref{fig:fusew}, we study the effect of scale fusion weight.

\begin{figure}
    \centering
    \includegraphics[width=0.8\columnwidth]{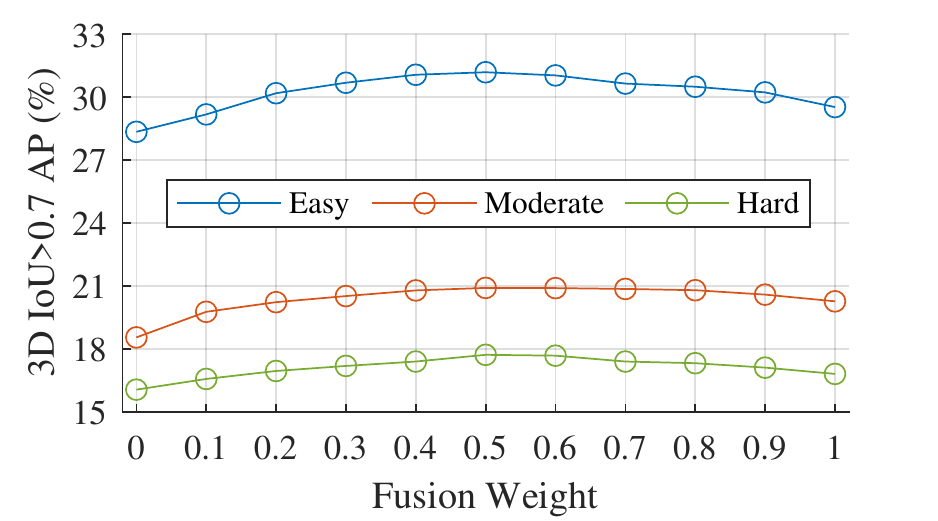}
    \caption{\textbf{Effect of Fusion Weight.} Lower weight value indicates lower impact from direct depth estimation and higher impact from scale in PnP solution.}
    \label{fig:fusew}
\end{figure}

%All these time are only for 3D localization that assumes given 2D detection.

\noindent \textbf{Visual scope.}
In the main paper we have studied the behavior of object-centric and scene-centric training in NeurOCS with NeRF. Here, we study the performance when training NOCS with Lidar directly without using NeRF-rendered supervision. This allows us to focus on the image-conditioned regression branch, although we observe the NeRF branch behaves similarly in the two schemes. The results are shown in \cref{table:objectscenecentric}. In addition to the vanilla scene-centric scheme, we replace its NOCS map prediction with the one from object-centric scheme, while keeping its object mask and score prediction; this setting is denoted as ``scene-centric++". As can be seen, while a performance gap exists between the object-centric and scene-centric training, scene-centric++ largely reduces the gap especially for the Moderate and Hard cases. This demonstrates the benefits of object-centric training towards more accurate NOCS map predictions. We also increase the network capacity in the scene-centric NOCS regression head by doubling its number of layers, but do not observe consistent improvements, as shown in ``scene-centric-L". Furthermore, we evaluate scene-centric scheme with DLA as the backbone, and similar results are observed.

\begin{table}
    \centering
    
    \resizebox{1.0\columnwidth}{!}{%
        % Please add the following required packages to your document preamble:
% \usepackage{multirow}

\begin{tabular}{c|ccc|ccc}
\hline
 \multicolumn{1}{c|}{\multirow{2}{*}{}}                               & \multicolumn{3}{c|}{PnP Only}                                       & \multicolumn{3}{c}{+ Fusion}                                       \\ 
 \multicolumn{1}{c|}{}                                                & Easy                 & Moderate             & Hard                  & Easy                 & Moderate             & Hard                 \\ \hline
%\multicolumn{1}{c|}{\multirow{3}{*}{NeurOCS}} & object-centric &   28.46 & 18.68 & 16.22 & 31.18 & 20.90 & 17.71  \\ \cline{2-8} 
%\multicolumn{1}{c|}{}                     & \renewcommand\arraystretch{0.8}\begin{tabular}[c]{@{}c@{}}scene-centric\\ (resnet)\end{tabular} &   24.28 & 16.57 & 13.63 & 28.11  & 19.17 & 16.32 \\ \cline{2-8} 
%\multicolumn{1}{c|}{}                     &   \renewcommand\arraystretch{0.8}\begin{tabular}[c]{@{}c@{}}scene-centric\\ (dla)\end{tabular} &  23.05 & 15.42  & 12.51  & 26.87 & 18.23 & 15.00           \\ \hline
 object-centric &  27.92 & 18.49 & 15.78 & 31.24 &21.01 & 17.70 \\ \hline 
 \begin{tabular}[c]{@{}c@{}}scene-centric\\ (resnet)\end{tabular}  &  26.39 &17.62 & 14.61 & 29.40 & 20.20 & 16.94 \\ \hline 
 
\begin{tabular}[c]{@{}c@{}}scene-centric++\\ (resnet)\end{tabular}& 25.30 & 18.02 & 15.64 & 28.54 & 20.60 & 17.57 \\ \hline 

\begin{tabular}[c]{@{}c@{}}scene-centric-L\\ (resnet)\end{tabular}& 25.95 & 17.35 & 14.51 & 29.57 & 20.39 & 17.06  \\ \hline  

\begin{tabular}[c]{@{}c@{}}scene-centric\\ (dla)\end{tabular} & 25.04 & 16.89 & 14.03 & 28.48 & 19.34 & 16.26\\ \hline 

\begin{tabular}[c]{@{}c@{}}scene-centric++\\ (dla)\end{tabular} & 26.00 & 18.05 & 15.81 & 29.25 & 20.60 & 17.55   \\ \hline

\end{tabular}
}
    \caption{Additional study on the benefits of object-centric training.}
    \label{table:objectscenecentric}
\end{table}

%\noindent \textbf{Bi-directional consistency.} The ablation study in main paper shows slight AP improvements by enforcing the bi-directional NOCS consistency (i.e. optimizing NeRF through the NOCS consistency loss). While its impact is relatively small, we observe that the bi-directional consistency may lead to slightly smoother and more structured shapes, with a few examples shown in \cref{fig:bidir}.
%We attach its qualitative result in Fig.\ref{fig:bidir}, showing slightly smoother and ordered shape at circled regions. 

\noindent \textbf{Uncertainty map.} As aforementioned, we learn a uncertain map for NOCS predictions using the reprojection loss, for both our w/ NeRF settings (NeurOCS) and those w/o NeRF baselines. We found that including the uncertainty map in the weight of PnP optimization improves the final performance. Here, we report in \cref{table:withoutuncertainty} the accuracy of NeurOCS in the case of without using it. 

\begin{table}[t]
    \centering
    
    \resizebox{1.0\columnwidth}{!}{%
        
\begin{tabular}{l|ccc|ccc}
\hline
 \multicolumn{1}{c|}{\multirow{2}{*}{}}                               & \multicolumn{3}{c|}{PnP only}                                       & \multicolumn{3}{c}{+ Fusion}                                       \\ 
 \multicolumn{1}{c|}{}                                                & Easy                 & Moderate             & Hard                  & Easy                 & Moderate             & Hard                 \\ \hline
 NeurOCS-MLC &  28.06 & 18.52 & 15.36 & 31.20 & 20.99 & 17.55\\ 
 NeurOCS-ML  &  28.23 & 18.58 & 15.49 & 30.79 & 20.80 & 17.48\\ 
 NeurOCS-MC  &  28.07 & 18.69 & 15.82 & 30.93 & 20.87 & 17.46\\ 
 NeurOCS-M   &  27.66 & 18.42 & 15.54 & 30.66 & 20.77 & 17.49\\
 \hline
\end{tabular}
}
    \caption{$AP_{3D}$ from NeurOCS without using the uncertainty map.}
    \label{table:withoutuncertainty}
\end{table}

\noindent \textbf{Note on NeRF.} While the shape rendering from NeRF is only required during training, we observe that it also works well for the validation set. We demonstrate this in \cref{fig:nerfshape} with an example object instance from the validation set.

\begin{figure}[t]
  \centering
  \includegraphics[width=1.0\linewidth, trim = 0mm 122mm 50mm 0mm, clip]{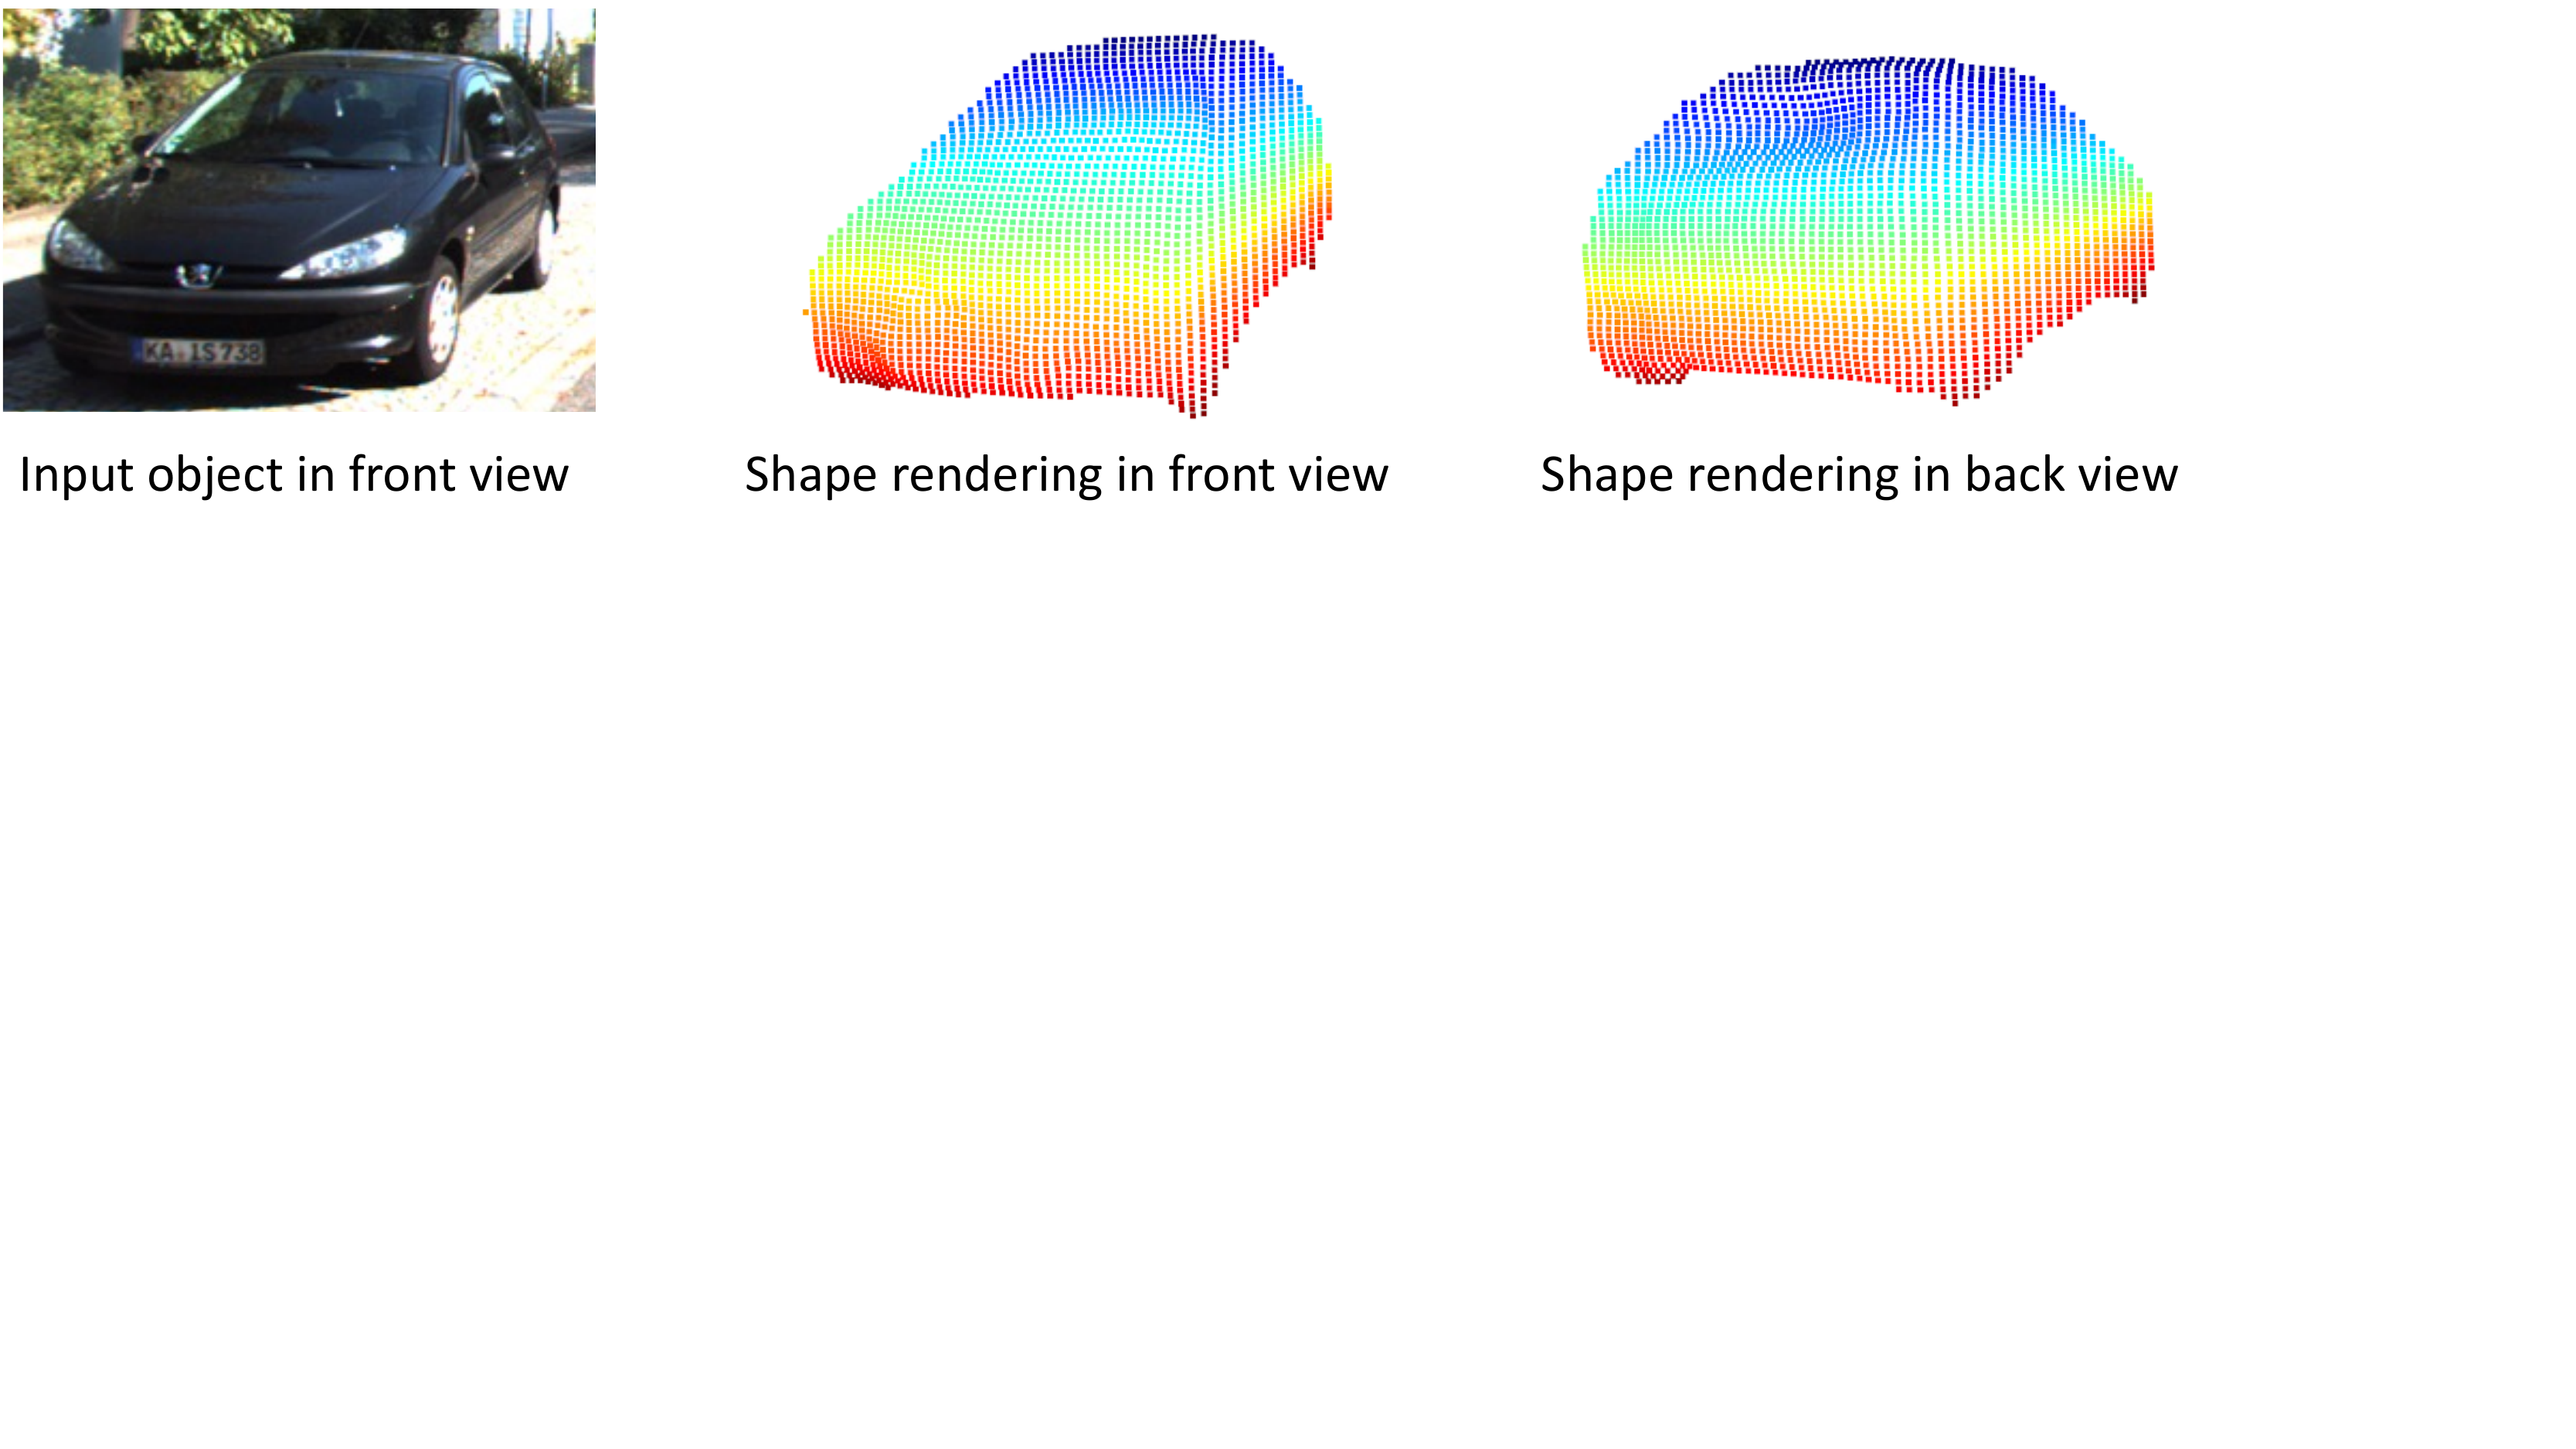}
  \centering
  \caption{Shape visualization for an example object instance from the validation set.}
  \label{fig:nerfshape}  
\end{figure}

\noindent \textbf{Qualitative results.} We demonstrate the output of NeurOCS by running on KITTI raw sequences that have no overlap with the training set. In particular, the sequences are from the KITTI-Tracking subset where ground truth 3D boxes are provided for every frame. These results are shown in the attached supplementary video.

\begin{table}[t]
\centering

\resizebox{1.0\columnwidth}{!}{
\begin{tabular}{l|ccc|ccc}
\hline
                             & \multicolumn{3}{c|}{DID-M3D} & \multicolumn{3}{c}{NeurOCS-MLC} \\ \cline{2-7} 
\multirow{2}{*}{Pedestraian} & Easy    & Moderate   & Hard  & Easy     & Moderate    & Hard   \\
                             & 11.27   & 8.75       & 7.15  & 12.13    & 9.21        & 7.40   \\ \hline
\end{tabular}}
\caption{$AP_{3D}$ on the pedestrian class in KITTI validation set.}
\label{table:pedestrian}
\end{table}

\noindent \textbf{Other object classes.} We report in \cref{table:pedestrian} the results on the pedestrian class; we omit cyclists as their instance masks are not provided by~\cite{heylen2021monocinis}. As shown, NeurOCS improves upon its base detector DID-M3D despite the non-rigid object topology, further indicating its robustness.

\noindent \textbf{Computation efficiency.}\label{sec:supp_runtime}
The runtime of our framework without TTA costs 50ms on average for each frame in KITTI object dataset on a single RTX2080. The ResNet50 backbone takes about 15ms and the pose solver costs 35ms, while the TTA doubles the backbone runtime.

\subsection{Evaluation on Waymo}
\begin{table}[t]
\centering
\vspace{-0.2cm}

\resizebox{1.0\columnwidth}{!}{

\begin{tabular}{c|c|cccc|cccc}
\hline
\multirow{2}{*}{Difficulty} & \multirow{2}{*}{Method} & \multicolumn{4}{c|}{$AP_{3D}$}                          & \multicolumn{4}{c}{$APH_{3D}$}                           \\ \cline{3-10} 
                            &                         & \multicolumn{1}{c|}{All}  & 0-30m & 30-50m & 50m-$\infty$ & \multicolumn{1}{c|}{All}  & 0-30m & 30-50m & 50m-$\infty$ \\ \hline
\multirow{5}{*}{Level\_1}     & PCT~\cite{wang2021progressive}                     & \multicolumn{1}{c|}{0.89} & 3.18  & 0.27   & 0.07 & \multicolumn{1}{c|}{0.88} & 3.15  & 0.27   & 0.07 \\
                            & MonoJSG~\cite{lian2022monojsg}                 & \multicolumn{1}{c|}{0.97} & 4.65  & 0.55   & 0.10 & \multicolumn{1}{c|}{0.95} & 4.59  & 0.53   & 0.09 \\
                            & DEVIANT~\cite{kumar2022deviant}                 & \multicolumn{1}{c|}{2.69} & 6.95  & 0.99   & 0.02 & \multicolumn{1}{c|}{2.67} & 6.90  & 0.98   & 0.02 \\ \cline{2-10} 
                            & NeurOCS (PnP)           & \multicolumn{1}{c|}{1.67} & 4.28  & 0.74   & 0.02 & \multicolumn{1}{c|}{1.66} & 4.26  & 0.73   & 0.02 \\
                            & NeurOCS (Fusion)        & \multicolumn{1}{c|}{2.44} & 6.35  & 0.97   & 0.04 & \multicolumn{1}{c|}{2.43} & 6.31  & 0.97   & 0.04 \\ \hline
\multirow{5}{*}{Level\_2}     & PCT~\cite{wang2021progressive}                     & \multicolumn{1}{c|}{0.66} & 3.18  & 0.27   & 0.07 & \multicolumn{1}{c|}{0.66} & 3.15  & 0.26   & 0.07 \\
                            & MonoJSG~\cite{lian2022monojsg}                 & \multicolumn{1}{c|}{0.91} & 4.64  & 0.55   & 0.09 & \multicolumn{1}{c|}{0.89} & 4.65  & 0.53   & 0.09 \\
                            & DEVIANT~\cite{kumar2022deviant}                 & \multicolumn{1}{c|}{2.52} & 6.93  & 0.95   & 0.02 & \multicolumn{1}{c|}{2.50} & 6.87  & 0.94   & 0.02 \\ \cline{2-10} 
                            & NeurOCS (PnP)           & \multicolumn{1}{c|}{1.56} & 4.26  & 0.71   & 0.02 & \multicolumn{1}{c|}{1.55} & 4.24  & 0.70   & 0.02 \\
                            & NeurOCS (Fusion)        & \multicolumn{1}{c|}{2.29} & 6.32  & 0.94   & 0.03 & \multicolumn{1}{c|}{2.28} & 6.29  & 0.93   & 0.03 \\ \hline
\end{tabular}
}
\caption{Evaluation on Waymo dataset with $IoU{\ge}0.7$.}
\label{tab:waymo}
\vspace{-0.2cm}
\end{table}

Here, we follow~\cite{kumar2022deviant,lian2022monojsg,wang2021progressive} to train on the Waymo~\cite{Sun_2020_CVPR} dataset, only using its front camera for the monocular 3D detection task.
The Waymo dataset contains 798 training sequences and 202 validation sequences, each with around 200 images. The objects are split into two difficulty level: ``Level\_1" and ``Level\_2", depending on the number of Lidar points within the object bounding box. For evaluation, we adopt the official metrics - 3D average precision $AP_{3D}$ and 3D average precision weighted by heading $APH_{3D}$. Besides evaluating all objects together, we also evaluate for objects separately in different distance ranges, including 0-30m, 30-50m, and 50m-$\infty$. We use the panoptic annotations in Waymo to extract instance masks, which are however provided only for a subset of images - as a result we train with 12128 images instead of 52386 as in \cite{kumar2022deviant,lian2022monojsg,wang2021progressive}.  Since DID-M3D~\cite{peng2022did} does not release the code for Waymo, we instead use DEVIANT~\cite{kumar2022deviant} as our base 3D detector. As shown in \cref{tab:waymo}, despite slightly lagging behind \cite{kumar2022deviant}, our method overall outperforms other recent methods~\cite{lian2022monojsg,wang2021progressive} even without fusion. This indicates the promising potential of our method towards 3D detection in more diverse and complex environment. Empirically, we observe that the 3D object bounding box annotations in Waymo are often not tight. This may affect the learning on object size and further on the localization accuracy of NeurOCS, since the object size directly impacts the object distance in the PnP optimization. Further, the rolling shutter effect~\cite{zhuang2017rolling} in the camera used by Waymo may impact our geometric optimization which  assumes the image is taken from a global shutter camera. We leave the handling of these challenges for performance improvements as the future work. 

%We applied the same training setup as in KITTI, but envision improved performance with adaptations, \eg increasing model capacity, which are omitted due to the time constraint during rebuttal.

\subsection{Evaluation on NuScenes}

\begin{table}[t]
    \centering
    
    \resizebox{1.0\columnwidth}{!}{%
        
\begin{tabular}{c|ccc|ccc}
 & \multicolumn{3}{c|}{Mean Depth MAE}& \multicolumn{3}{c}{Median Depth MAE}\\ \hline
\begin{tabular}[c]{@{}c@{}}range\\ (\# of obj.)\end{tabular} & \begin{tabular}[c]{@{}c@{}}0-20m\\ (596)\end{tabular} & \begin{tabular}[c]{@{}c@{}}20-40m\\ (719)\end{tabular} & \begin{tabular}[c]{@{}c@{}}\textgreater{}40m\\ (16)\end{tabular} & \begin{tabular}[c]{@{}c@{}}0-20m\\ (596)\end{tabular} & \begin{tabular}[c]{@{}c@{}}20-40m\\ (719)\end{tabular} & \begin{tabular}[c]{@{}c@{}}\textgreater{}40m\\ (16)\end{tabular} \\ \hline
DEVIANT~\cite{kumar2022deviant}   & 0.757  & \textbf{1.603}    & \textbf{4.499}   & 0.660  & 1.270  & \textbf{4.590}  \\ 
NeurOCS-PnP  & 0.746  & 2.160    & 6.719   & 0.575  & 1.780  & 6.725  \\ 
NeurOCS-Fusion & \textbf{0.602}   & 1.714    & 5.624   & \textbf{0.460}  & \textbf{1.180}  & 5.415 \\ \hline \hline

\begin{tabular}[c]{@{}c@{}}range\\ (\# of obj.)\end{tabular} & \begin{tabular}[c]{@{}c@{}}0-20m\\ (1273)\end{tabular} & \begin{tabular}[c]{@{}c@{}}20-40m\\ (2173)\end{tabular} & \begin{tabular}[c]{@{}c@{}}\textgreater{}40m\\ (858)\end{tabular} & \begin{tabular}[c]{@{}c@{}}0-20m\\ (1273)\end{tabular} & \begin{tabular}[c]{@{}c@{}}20-40m\\ (2173)\end{tabular} & \begin{tabular}[c]{@{}c@{}}\textgreater{}40m\\ (858)\end{tabular} \\ \hline
DID-M3D~\cite{peng2022did}   & 0.665  & \textbf{1.713}    & \textbf{3.373}   & 0.510  & 1.400  & \textbf{2.740}  \\ 
NeurOCS-PnP   & 0.801  & 2.396    & 5.671   & 0.650  & 1.950  & 5.275  \\ 
NeurOCS-Fusion   & \textbf{0.637}  & 1.721    & 3.711   & \textbf{0.480} & \textbf{1.380}  & 3.150  \\ 

\end{tabular}

    }
    \caption{\textbf{Cross-dataset evaluation on NuScenes.} The depth MAEs are reported for recalled objects in different ranges, each containing \# objects as shown.}
    \label{table:nuscenes_deviant}
\end{table}

While cross-dataset generalization is not the main goal of our work, we follow DEVIANT~\cite{kumar2022deviant} to perform evaluation in NuScenes dataset~\cite{caesar2020nuscenes} to understand its generalization capability.  Specifically, we train on the training split of the KITTI training set and evaluate on all 6019 frontal images in the NuScenes validation set, using the mean absolute error (MAE)~\cite{kumar2022deviant,shi2021geometry} of the depth of the boxes. This is computed only on recalled objects (2D IoU$>
$0.7) where the ground truth depth can be retrieved; strictly speaking, the 3D error measured by depth MAE from two methods are comparable only when using the same set of recalled objects. We first compare with DEVIANT as shown in \cref{table:nuscenes_deviant}, where we use DEVIANT as our base detector to have the same set of recalled objects. As can be seen, while DEVIANT achieves good performance due to its special design in depth-equivariant architecture, NeurOCS yields reasonable performance with PnP alone, and its fusion with DEVIANT leads to improvements in some cases especially for nearby objects. Similar observations are obtained when using DID-M3D as the base detector. These results indicate the promising potential of NeurOCS in generalization due to its underlying geometric principles, especially for the near field where the PnP solution is less sensitive to the error in object size prediction. Further explorations towards improving its generalization capability remain our future work.
