# Supplementary material for: NeurOCS: Neural NOCS Supervision for Monocular 3D Object Localization
Source: arXiv:2305.17763 source file (2023-05-28)
Supplement: Supplementary file 3 [file supp_ablation_network_arch.tex]

\begin{tabular}{c|c|ccc|ccc}
\hline
\multirow{2}{*}{Module} & \multirow{2}{*}{Model} & \multicolumn{3}{c|}{PnP Only} & \multicolumn{3}{c}{+ Fusion} \\ \cline{3-8} 
 &  & Easy & Moderate & Hard & Easy & Moderate & Hard \\ \hline
 \multirow{1}{*}{Default} & ResNet50+5 Grid Scales & 27.92 & 18.49 & 15.78 & 31.24 &21.01 & 17.70 \\ \hline
 \multirow{2}{*}{Backbone} & ResNet18 & 27.04 & 18.21 & 15.39 & 30.18 & 20.80 & 17.44 \\
 & ResNet34 & 27.00 & 18.19 & 15.47 & 30.39 & 20.71 & 17.38\\ \hline
\multirow{3}{*}{NeRF} & 4 Grid Scales & 27.80 & 18.49 & 15.81 & 30.93 & 20.90 & 17.56\\
 & 3 Grid Scales & 28.02 & 18.62 & 15.89 & 31.16 & 21.02 & 17.64\\
 & CodeNeRF & 27.41 & 18.23 & 15.10 & 30.53 & 20.77 & 17.45  \\ \hline
\end{tabular}
