# Supplementary material for: NeurOCS: Neural NOCS Supervision for Monocular 3D Object Localization
Source: arXiv:2305.17763 source file (2023-05-28)
Supplement: Supplementary file 4 [file supp_comparewith_cmkd.tex]

\begin{tabular}{l|c|lll|lll}
\multirow{2}{*}{Method} & \multirow{2}{*}{Venue} & \multicolumn{3}{c|}{3D $AP_{40} $ - Test} & \multicolumn{3}{c}{BEV $AP_{40} $ - Test} \\ \cline{3-8} 
                        &                        & Easy       & Mod      & Hard      & Easy      & Mod      & Hard      \\ \hline
                      LPCG~\cite{peng2022lidar}  & ECCV22 & 25.56 & 17.80 & 15.38 & 35.96 & 24.81 & 21.86  \\
                      CMKD~\cite{hong2022cross} & ECCV22 & 28.55 & 18.69 & 16.77 & 38.98 & 25.82 & 22.80 \\
                      NeurOCS  & CVPR23 &  29.89 & 18.94 & 15.90 & 37.27 & 24.49 & 20.89
\end{tabular}
