# Supplementary material for: NeurOCS: Neural NOCS Supervision for Monocular 3D Object Localization
Source: arXiv:2305.17763 source file (2023-05-28)
Supplement: Supplementary file 5 [file supp_comparewith_deviant.tex]

\begin{tabular}{c|c|lll|lll}
\multirow{2}{*}{Method} & \multirow{2}{*}{Venue} & \multicolumn{3}{c|}{3D $AP_{40} $ - Val} & \multicolumn{3}{c}{BEV $AP_{40} $ - Val} \\ \cline{3-8} 
                        &                        & Easy       & Mod      &Hard      & Easy      & Mod      & Hard      \\ \hline
DEVIANT~\cite{kumar2022deviant}  & ECCV22 &  25.09 & 16.99 & 15.30 & 33.69 & 23.10 & 20.67           \\\hline
%NeurOCS-M   & - & 22.71 & 15.78 & 14.01 & 29.32 & 21.40 &  18.79 \\
%NeurOCS-MLC  & - & 21.98& 15.73 & 13.79 & 29.33 & 21.22 & 18.64 %\\\hline    
NeurOCS-M + \cite{kumar2022deviant}  & CVPR23 & 27.70 & 18.92 & 16.28 & 35.31 & 25.11 & 21.87 \\        
NeurOCS-MLC + \cite{kumar2022deviant}  & CVPR23 & 27.83 & 18.92 & 16.20 & 35.14 & 24.77 & 21.43 \\        
\end{tabular}
