# Supplementary material for: NeurOCS: Neural NOCS Supervision for Monocular 3D Object Localization
Source: arXiv:2305.17763 source file (2023-05-28)
Supplement: Supplementary file 6 [file supp_losses.tex]

\begin{tabular}{c|c|c|c|c|c}
\hline
Module & Loss Name & Type & Weight & Region & Note \\ \hline
\multirow{6}{*}{NeRF} & Occupancy Loss & L2 & 1 & FG + BG &  \\
 & RGB Loss & L2 & 3 & FG &  \\
 & KL Divergence & KL & 1 & - &  \\
 & Lidar Loss & L2 & 0.5 & FG \& Valid & Optional \\
 & LiComp Loss & L2 & 0.2 & FG \& Valid & Optional \\
 & Dense Prior & L1 & 0.002 & 3D Grid & Conditional \\ \hline
\multirow{3}{*}{Image} & FG Loss & L2 & 1 & All &  \\
 & IoU Score Loss & L2 & 1 & - &  \\
 & Reproj. Loss & L2 & 2 & FG &  \\ \hline
Both & NOCS Consistency & L2 & 1 & FG \& Occ &  \\ \hline

\multicolumn{6}{r}{\small {FG = Foreground, \; BG = Backgroud}}

\end{tabular}
