# Supplementary material for: NeurOCS: Neural NOCS Supervision for Monocular 3D Object Localization
Source: arXiv:2305.17763 source file (2023-05-28)
Supplement: Supplementary file 7 [file supp_nuscenes_deviant.tex]

\begin{tabular}{c|ccc|ccc}
 & \multicolumn{3}{c|}{Mean Depth MAE}& \multicolumn{3}{c}{Median Depth MAE}\\ \hline
\begin{tabular}[c]{@{}c@{}}range\\ (\# of obj.)\end{tabular} & \begin{tabular}[c]{@{}c@{}}0-20m\\ (596)\end{tabular} & \begin{tabular}[c]{@{}c@{}}20-40m\\ (719)\end{tabular} & \begin{tabular}[c]{@{}c@{}}\textgreater{}40m\\ (16)\end{tabular} & \begin{tabular}[c]{@{}c@{}}0-20m\\ (596)\end{tabular} & \begin{tabular}[c]{@{}c@{}}20-40m\\ (719)\end{tabular} & \begin{tabular}[c]{@{}c@{}}\textgreater{}40m\\ (16)\end{tabular} \\ \hline
DEVIANT~\cite{kumar2022deviant}   & 0.757  & \textbf{1.603}    & \textbf{4.499}   & 0.660  & 1.270  & \textbf{4.590}  \\ 
NeurOCS-PnP  & 0.746  & 2.160    & 6.719   & 0.575  & 1.780  & 6.725  \\ 
NeurOCS-Fusion & \textbf{0.602}   & 1.714    & 5.624   & \textbf{0.460}  & \textbf{1.180}  & 5.415 \\ \hline \hline

\begin{tabular}[c]{@{}c@{}}range\\ (\# of obj.)\end{tabular} & \begin{tabular}[c]{@{}c@{}}0-20m\\ (1273)\end{tabular} & \begin{tabular}[c]{@{}c@{}}20-40m\\ (2173)\end{tabular} & \begin{tabular}[c]{@{}c@{}}\textgreater{}40m\\ (858)\end{tabular} & \begin{tabular}[c]{@{}c@{}}0-20m\\ (1273)\end{tabular} & \begin{tabular}[c]{@{}c@{}}20-40m\\ (2173)\end{tabular} & \begin{tabular}[c]{@{}c@{}}\textgreater{}40m\\ (858)\end{tabular} \\ \hline
DID-M3D~\cite{peng2022did}   & 0.665  & \textbf{1.713}    & \textbf{3.373}   & 0.510  & 1.400  & \textbf{2.740}  \\ 
NeurOCS-PnP   & 0.801  & 2.396    & 5.671   & 0.650  & 1.950  & 5.275  \\ 
NeurOCS-Fusion   & \textbf{0.637}  & 1.721    & 3.711   & \textbf{0.480} & \textbf{1.380}  & 3.150  \\ 

\end{tabular}
