# Supplementary material for: NeurOCS: Neural NOCS Supervision for Monocular 3D Object Localization
Source: arXiv:2305.17763 source file (2023-05-28)
Supplement: Supplementary file 8 [file supp_objectscenecentric.tex]

% Please add the following required packages to your document preamble:
% \usepackage{multirow}

\begin{tabular}{c|ccc|ccc}
\hline
 \multicolumn{1}{c|}{\multirow{2}{*}{}}                               & \multicolumn{3}{c|}{PnP Only}                                       & \multicolumn{3}{c}{+ Fusion}                                       \\ 
 \multicolumn{1}{c|}{}                                                & Easy                 & Moderate             & Hard                  & Easy                 & Moderate             & Hard                 \\ \hline
%\multicolumn{1}{c|}{\multirow{3}{*}{NeurOCS}} & object-centric &   28.46 & 18.68 & 16.22 & 31.18 & 20.90 & 17.71  \\ \cline{2-8} 
%\multicolumn{1}{c|}{}                     & \renewcommand\arraystretch{0.8}\begin{tabular}[c]{@{}c@{}}scene-centric\\ (resnet)\end{tabular} &   24.28 & 16.57 & 13.63 & 28.11  & 19.17 & 16.32 \\ \cline{2-8} 
%\multicolumn{1}{c|}{}                     &   \renewcommand\arraystretch{0.8}\begin{tabular}[c]{@{}c@{}}scene-centric\\ (dla)\end{tabular} &  23.05 & 15.42  & 12.51  & 26.87 & 18.23 & 15.00           \\ \hline
 object-centric &  27.92 & 18.49 & 15.78 & 31.24 &21.01 & 17.70 \\ \hline 
 \begin{tabular}[c]{@{}c@{}}scene-centric\\ (resnet)\end{tabular}  &  26.39 &17.62 & 14.61 & 29.40 & 20.20 & 16.94 \\ \hline 
 
\begin{tabular}[c]{@{}c@{}}scene-centric++\\ (resnet)\end{tabular}& 25.30 & 18.02 & 15.64 & 28.54 & 20.60 & 17.57 \\ \hline 

\begin{tabular}[c]{@{}c@{}}scene-centric-L\\ (resnet)\end{tabular}& 25.95 & 17.35 & 14.51 & 29.57 & 20.39 & 17.06  \\ \hline  

\begin{tabular}[c]{@{}c@{}}scene-centric\\ (dla)\end{tabular} & 25.04 & 16.89 & 14.03 & 28.48 & 19.34 & 16.26\\ \hline 

\begin{tabular}[c]{@{}c@{}}scene-centric++\\ (dla)\end{tabular} & 26.00 & 18.05 & 15.81 & 29.25 & 20.60 & 17.55   \\ \hline

\end{tabular}
