# Supplementary material for: NeurOCS: Neural NOCS Supervision for Monocular 3D Object Localization
Source: arXiv:2305.17763 source file (2023-05-28)
Supplement: Supplementary file 9 [file supp_withoutnerf.tex]

% Please add the following required packages to your document preamble:
% \usepackage{multirow}

\begin{tabular}{l|ccc|ccc}
\hline
 \multicolumn{1}{c|}{\multirow{2}{*}{}}                               & \multicolumn{3}{c|}{PnP Only}                                       & \multicolumn{3}{c}{+ Fusion}                                       \\ 
 \multicolumn{1}{c|}{}                                                & Easy                 & Moderate             & Hard                  & Easy                 & Moderate             & Hard                 \\ \hline
 RLC & 27.55 & 18.27 & 15.75 & 30.79 & 20.78 & 17.37   \\ 
 RL &  27.50 & 18.36 & 15.77 & 30.45 & 20.71 & 17.45 \\ 
 RC &  27.08 & 18.10 & 15.28 & 30.74 & 20.67 & 17.41 \\ 
 R &   22.59 & 15.81 & 13.07 & 27.26 & 19.10 & 16.48\\
 \hline
\end{tabular}
