# Supplementary material for: NeurOCS: Neural NOCS Supervision for Monocular 3D Object Localization
Source: arXiv:2305.17763 source file (2023-05-28)
Supplement: Supplementary file 10 [file supp_withoutuncertainty.tex]

\begin{tabular}{l|ccc|ccc}
\hline
 \multicolumn{1}{c|}{\multirow{2}{*}{}}                               & \multicolumn{3}{c|}{PnP only}                                       & \multicolumn{3}{c}{+ Fusion}                                       \\ 
 \multicolumn{1}{c|}{}                                                & Easy                 & Moderate             & Hard                  & Easy                 & Moderate             & Hard                 \\ \hline
 NeurOCS-MLC &  28.06 & 18.52 & 15.36 & 31.20 & 20.99 & 17.55\\ 
 NeurOCS-ML  &  28.23 & 18.58 & 15.49 & 30.79 & 20.80 & 17.48\\ 
 NeurOCS-MC  &  28.07 & 18.69 & 15.82 & 30.93 & 20.87 & 17.46\\ 
 NeurOCS-M   &  27.66 & 18.42 & 15.54 & 30.66 & 20.77 & 17.49\\
 \hline
\end{tabular}
