# Supplementary material for: NeurOCS: Neural NOCS Supervision for Monocular 3D Object Localization
Source: arXiv:2305.17763 source file (2023-05-28)
Supplement: Supplementary file 11 [file BACKUP_supp_objectscenecentric.tex]

% Please add the following required packages to your document preamble:
% \usepackage{multirow}
\renewcommand\arraystretch{2.0}
\begin{tabular}{cl|ccc|ccc}
\hline
\multicolumn{1}{l}{}                      & \multicolumn{1}{c|}{\multirow{2}{*}{}}                               & \multicolumn{3}{c|}{PnP Only}                                       & \multicolumn{3}{c}{+ Fusion}                                       \\ \cline{3-8} 
\multicolumn{1}{l}{}                      & \multicolumn{1}{c|}{}                                                & Easy                 & Moderate             & Hard                  & Easy                 & Moderate             & Hard                 \\ \hline
%\multicolumn{1}{c|}{\multirow{3}{*}{NeurOCS}} & object-centric &   28.46 & 18.68 & 16.22 & 31.18 & 20.90 & 17.71  \\ \cline{2-8} 
%\multicolumn{1}{c|}{}                     & \renewcommand\arraystretch{0.8}\begin{tabular}[c]{@{}c@{}}scene-centric\\ (resnet)\end{tabular} &   24.28 & 16.57 & 13.63 & 28.11  & 19.17 & 16.32 \\ \cline{2-8} 
%\multicolumn{1}{c|}{}                     &   \renewcommand\arraystretch{0.8}\begin{tabular}[c]{@{}c@{}}scene-centric\\ (dla)\end{tabular} &  23.05 & 15.42  & 12.51  & 26.87 & 18.23 & 15.00           \\ \hline
\multicolumn{1}{c|}{\multirow{6}{*}{\renewcommand\arraystretch{1.6}\begin{tabular}[c]{@{}c@{}} Lidar\end{tabular}}} & object-centric &  27.15  & 18.04 & 14.91 & 30.19 & 20.32 & 17.04 \\ \cline{2-8} 
\multicolumn{1}{c|}{}                     & \renewcommand\arraystretch{0.8}\begin{tabular}[c]{@{}c@{}}scene-centric\\ (resnet)\end{tabular}  &  25.89 & 17.14 & 14.37 & 28.53 & 19.48 &  16.65 \\ \cline{2-8} 
\multicolumn{1}{c|}{}& \renewcommand\arraystretch{0.8}\begin{tabular}[c]{@{}c@{}}scene-centric-L\\ (resnet)\end{tabular}& \multicolumn{1}{l}{24.71} & \multicolumn{1}{c}{16.20} & \multicolumn{1}{l|}{13.38} & \multicolumn{1}{l}{28.00} & \multicolumn{1}{c}{18.98} & \multicolumn{1}{l}{16.13} \\ \cline{2-8} 

\multicolumn{1}{c|}{}& \renewcommand\arraystretch{0.8}\begin{tabular}[c]{@{}c@{}}scene-centric++\\ (resnet)\end{tabular}& \multicolumn{1}{c}{26.53} & \multicolumn{1}{c}{17.91} & \multicolumn{1}{l|}{14.82} & \multicolumn{1}{l}{29.16} & \multicolumn{1}{c}{20.15} & \multicolumn{1}{l}{16.87} \\ \cline{2-8} 

\multicolumn{1}{c|}{}&\renewcommand\arraystretch{0.8}\begin{tabular}[c]{@{}c@{}}scene-centric\\ (dla)\end{tabular} &24.38 & 16.07  & 13.13 & 27.49 & 18.55 & 15.31  \\ \cline{2-8}

\multicolumn{1}{c|}{}&\renewcommand\arraystretch{0.8}\begin{tabular}[c]{@{}c@{}}scene-centric++\\ (dla)\end{tabular} & 26.23  & 17.82  & 14.82 & 29.05 & 20.12  & 16.97   \\ \hline


\multicolumn{1}{c|}{\multirow{5}{*}{\renewcommand\arraystretch{2.0}\begin{tabular}[c]{@{}c@{}}  \renewcommand\arraystretch{0.8}\begin{tabular}[c]{@{}c@{}}Lidar+\\ Lidar Comp.\end{tabular} \end{tabular}}} & object-centric & 28.01 & 18.39 & 15.63 & 30.42 & 20.58 & 17.23 \\ \cline{2-8} 

\multicolumn{1}{l|}{}&\renewcommand\arraystretch{0.8}\begin{tabular}[c]{@{}c@{}}scene-centric\\ (resnet)\end{tabular} &  26.23 & 16.76 & 14.05 & 28.33 & 19.12 & 16.03 \\ \cline{2-8} 

\multicolumn{1}{l|}{}&\renewcommand\arraystretch{0.8}\begin{tabular}[c]{@{}c@{}}scene-centric++\\ (resnet)\end{tabular} &  27.18 & 18.49 & 15.56  & 29.45 & 20.31 & 17.12 \\ \cline{2-8} 

\multicolumn{1}{l|}{}& \renewcommand\arraystretch{0.8}\begin{tabular}[c]{@{}c@{}}scene-centric\\ (dla)\end{tabular}& 24.16 &  16.01 & 13.03 & 28.08 &18.69 & 15.45 \\ \cline{2-8} 

\multicolumn{1}{l|}{}& \renewcommand\arraystretch{0.8}\begin{tabular}[c]{@{}c@{}}scene-centric++\\ (dla)\end{tabular}& 26.94  & 18.41  & 15.28  & 29.42 & 20.31 & 17.13 \\ \hline

\end{tabular}
